# Supplementary material for: EarGate: Gait-based User Identification with In-ear Microphones
Source: arXiv:2108.12305 source file (2021-08-27)
Supplement: Supplementary file 1 [file Appendix.tex]

\clearpage 
\section*{Appendix}

We present the detailed performance comparison of five typical machine learning classifiers (Logistic Regression-LR, Support Vector Machine-SVM, K Nearest Neighbours-KNN, Decision Tree-DT, and Random Forest-RF) on human activity recognition and hand-to-face gesture interaction.

\subsection*{Human Activity Recognition}
{\bf Overall performance: }
Figure~\ref{fig:har_5c_overall} compares the overall performance of the five classifiers with 5-fold cross-validation mechanism, which is basically an extended version of Figure~\ref{fig:har_overall}. We can observe that SVM, KNN, and RF obtain similar precision and recall. Although KNN and RF achieve slightly better performance on the left and right dataset, the highest precision and recall are acquired with SVM on the fused dataset. The performance of LR and DT is relatively worse on all the three datasets.

\begin{figure}[h]
	\centering
	\includegraphics[scale = 0.42]{fig/har_5c_overall.pdf}
	\vspace{-0.2in}
	\caption{Average activity recognition performance of the five classifiers.}
	\vspace{-0.1in}
	\label{fig:har_5c_overall}
\end{figure}

{\bf Individual performance: }Then, we compare the individual recognition recall for the leave-one-out test (fused dataset) among the five classifiers in Figure~\ref{fig:har_5c_ind_recall_concat}. We can see that different classifiers perform distinctively among different subjects. For example, LR performs the best for Subject 1, while RF achieves best recall for most subjects. Thus, the selection of classifiers should be personalized for users as well. The averaged recall with the classifiers is 84.3\% (LR), 79.7\% (SVM), 79.7\% (KNN), 75.1\% (DT), and 86.0\% (RF), respectively.

\begin{figure}[h]
	\centering
	\includegraphics[scale = 0.42]{fig/har_5c_ind_recall_concat.pdf}
	\vspace{-0.2in}
	\caption{Individual activity recognition recall of the five classifiers.}
	\vspace{-0.1in}
	\label{fig:har_5c_ind_recall_concat}
\end{figure}

\subsection*{Hand-to-face Gesture Interaction}
With the 12 gesture dataset, Figure~\ref{fig:ges_5c_ind_recall_concat} shows the comparison of individual recognition recall, where we can observe that the performance of different classifiers is consistent among subjects. Figure~\ref{fig:ges_5c_overall} compares the overall performance of the five classifiers on the 12 gestures. The results show that LR achieves the best performance, followed by RF with slightly lower precision and recall. SVM, KNN, and DT obtain similar performance but much lower than the other two classifiers. The results are consistent with the performance obtained on the 7 gesture set (Figure~\ref{fig:ges_5c_overall_7}) and 5 gesture set (Figure~\ref{fig:ges_5c_overall_5}).  

\begin{figure}[h]
	\centering
	\vspace{-0.1in}
	\includegraphics[scale = 0.42]{fig/ges_5c_ind_recall_concat.pdf}
	\vspace{-0.2in}
	\caption{Average gesture recognition performance of the five classifiers (12 gestures).}
	\vspace{-0.1in}
	\label{fig:ges_5c_ind_recall_concat}
\end{figure}

\begin{figure}[h]
	\centering
	\includegraphics[scale = 0.42]{fig/ges_5c_overall.pdf}
	\vspace{-0.2in}
	\caption{Individual gesture recognition performance of the five classifiers (12 gestures).}
	\vspace{-0.1in}
	\label{fig:ges_5c_overall}
\end{figure}

\begin{figure}[h]
	\centering
	\includegraphics[scale = 0.42]{fig/ges_5c_overall_7.pdf}
	\vspace{-0.2in}
	\caption{Individual gesture recognition performance of the five classifiers (7 gestures).}
	\vspace{-0.1in}
	\label{fig:ges_5c_overall_7}
\end{figure}

\begin{figure}[h]
	\centering
	\includegraphics[scale = 0.42]{fig/ges_5c_overall_5.pdf}
	\vspace{-0.2in}
	\caption{Individual gesture recognition performance of the five classifiers (5 gestures).}
	\vspace{-0.1in}
	\label{fig:ges_5c_overall_5}
\end{figure}
